# Supplementary material for: Implementation and benchmark of a long-range corrected functional in the density functional based tight-binding method
Source: arXiv:1504.00243 source file (2015-04-01)
Supplement: Supplementary file 1 [file SupportingInformation.pdf]

# — Supporting information —

# Implementation and benchmark of a long-range corrected functional in the density functional based tight-binding method

V. Lutsker,[†] B. Aradi,[‡] and T. A. Niehaus[*,†]

*Department of Theoretical Physics, University of Regensburg, 93040 Regensburg, Germany, and BCCMS, University of Bremen, 28359 Bremen, Germany*

E-mail: thomas.niehaus@physik.uni-regensburg.de

[*]To whom correspondence should be addressed

[†]Department of Theoretical Physics, University of Regensburg, 93040 Regensburg, Germany

[‡]BCCMS, University of Bremen, 28359 Bremen, Germany

# 1 Structural formulas for the compounds in the test set

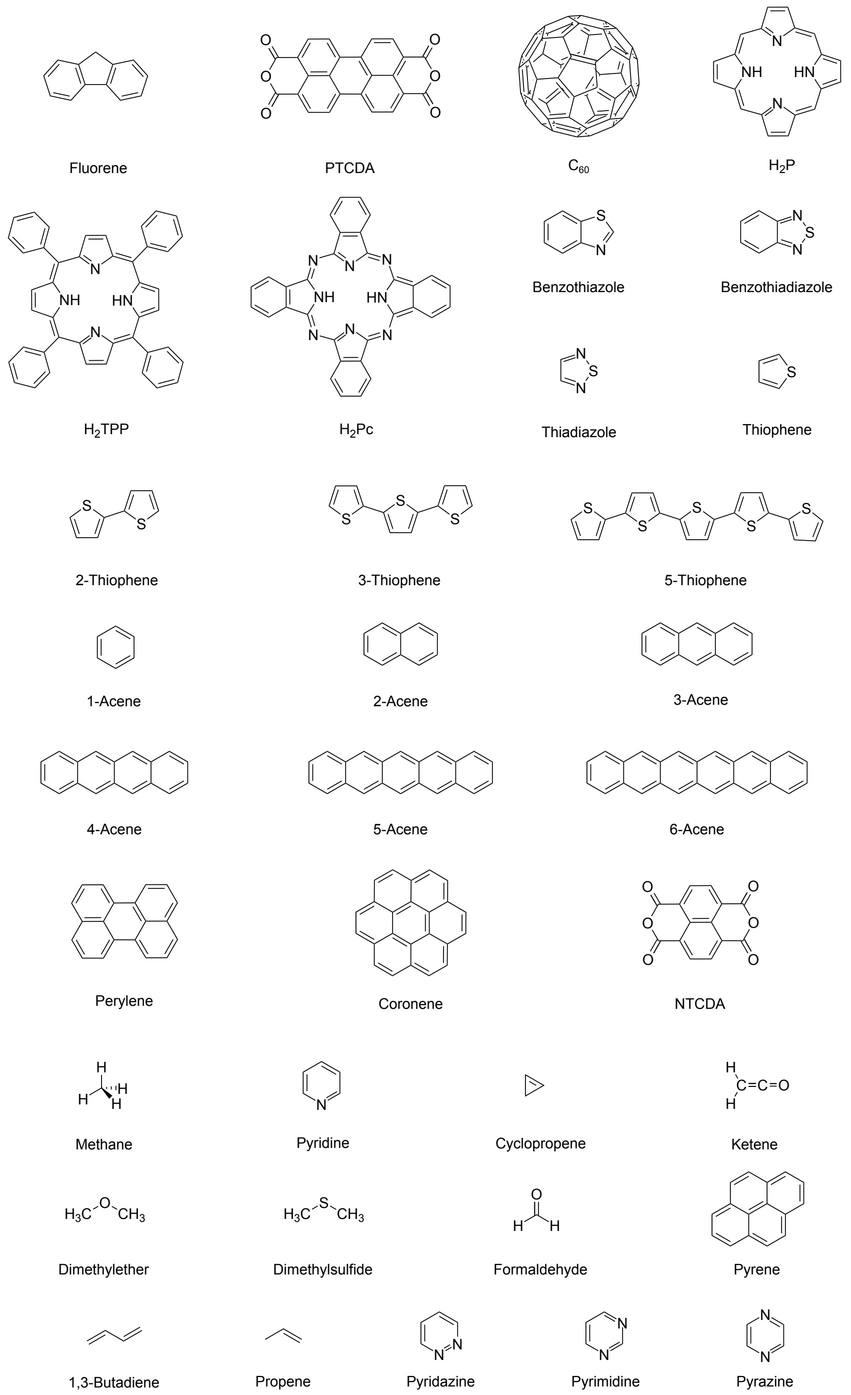


Figure S1: Structural formulas for the compounds in the test set.

# 2 Quasiparticle energies

Table S1: The negative of the HOMO eigenvalue for different theories compared to the experimental IP. All energies in eV.

| molecule | Exp | PBE/cc-pVTZ | B3LYP/cc-pVTZ | BNL/3-21G | BNL/cc-pVDZ | BNL/cc-pVTZ | LC-DFTB | DFTB |
|---|---|---|---|---|---|---|---|---|
| Fluorene | 7.91 | 5.40 | 7.02 | 7.68 | 7.81 | 7.97 | 8.08 | 5.89 |
| PTCDA | 8.20 | 6.30 | 6.88 | 7.84 | 8.05 | 8.32 | 8.46 | 6.41 |
| $C_{60}$ | 7.60 | 5.80 | 6.35 | 8.01 | 7.83 | 8.02 | 7.80 | 5.85 |
| $H_2P$ | 6.90 | 4.97 | 5.48 | 6.31 | 6.62 | 6.85 | 6.79 | 5.16 |
| $H_2TPP$ | 6.42 | 4.64 | 5.07 | 5.83 | 6.10 | 6.30 | 6.32 | 4.91 |
| $H_2Pc$ | 6.41 | 4.98 | 5.27 | 6.17 | 6.15 | 6.32 | 6.12 | 4.95 |
| Benzothiazole | 8.80 | 5.94 | 6.66 | 8.36 | 8.42 | 8.62 | 8.46 | 6.24 |
| Benzothiadiazole | 9.00 | 6.10 | 6.82 | 8.44 | 8.55 | 8.79 | 8.66 | 6.50 |
| Thiadiazole | 10.10 | 6.83 | 7.69 | 9.70 | 9.56 | 9.76 | 8.75 | 6.47 |
| Thiophene | 8.86 | 5.79 | 6.58 | 8.54 | 8.58 | 8.79 | 8.76 | 6.24 |
| 2-Thiophene | 7.75 | 5.00 | 5.66 | 7.40 | 7.43 | 7.62 | 7.85 | 5.52 |
| 3-Thiophene | 7.43 | 4.70 | 5.29 | 6.92 | 6.94 | 7.12 | 7.40 | 5.23 |
| 5-Thiophene | 7.11 | 4.47 | 4.99 | 6.53 | 6.54 | 6.71 | 6.79 | 5.00 |
| 1-Acene | 9.24 | 6.29 | 7.04 | 8.89 | 9.04 | 9.21 | 9.23 | 6.69 |
| 2-Acene | 8.14 | 5.44 | 6.09 | 7.70 | 7.87 | 8.04 | 8.22 | 5.98 |
| 3-Acene | 7.44 | 4.94 | 5.50 | 6.95 | 7.12 | 7.29 | 7.55 | 5.52 |
| 4-Acene | 6.97 | 4.61 | 5.12 | 6.44 | 6.62 | 6.78 | 7.10 | 5.22 |
| 5-Acene | 6.63 | 4.38 | 4.85 | 6.08 | 6.26 | 6.42 | 6.79 | 5.02 |
| 6-Acene | 6.40 | 4.23 | 4.66 | 5.82 | 6.00 | 6.15 | 6.57 | 4.88 |
| Perylene | 6.96 | 4.70 | 5.20 | 6.56 | 6.71 | 6.86 | 7.17 | 5.32 |
| Coronene | 7.29 | 5.21 | 5.74 | 7.11 | 7.24 | 7.39 | 7.63 | 5.71 |
| NTCDA | 9.67 | 6.84 | 8.04 | 9.20 | 9.42 | 9.73 | 9.33 | 6.79 |
| Methane | 12.61 | 9.43 | 10.76 | 12.62 | 12.74 | 12.90 | 11.79 | 9.14 |
| Pyridine | 9.26 | 5.77 | 7.09 | 8.23 | 8.78 | 9.06 | 8.39 | 6.21 |
| Cyclopropene | 9.67 | 5.94 | 6.86 | 8.74 | 8.86 | 9.03 | 8.74 | 6.29 |
| Ketene | 9.62 | 5.86 | 6.90 | 8.20 | 8.63 | 8.98 | 8.46 | 6.41 |
| Dimetylether | 10.03 | 5.63 | 7.06 | 7.98 | 8.64 | 9.02 | 8.24 | 5.89 |
| Dimethylsulfide | 8.69 | 5.05 | 6.06 | 7.92 | 7.90 | 8.13 | 7.99 | 5.69 |
| Formaldehyde | 10.88 | 6.17 | 7.56 | 8.61 | 9.02 | 9.41 | 8.61 | 6.36 |
| Pyrene | 7.43 | 5.06 | 5.61 | 7.00 | 7.17 | 7.33 | 7.56 | 5.59 |
| 1,3-Butadiene | 9.07 | 5.79 | 6.55 | 8.31 | 8.54 | 8.73 | 8.97 | 6.44 |
| Propene | 9.73 | 6.14 | 7.04 | 8.94 | 9.14 | 9.33 | 9.40 | 6.78 |
| Pyridazine | 8.74 | 5.24 | 6.61 | 7.55 | 8.19 | 8.53 | 7.89 | 5.72 |
| Pyrimidine | 9.33 | 5.73 | 7.04 | 8.27 | 8.74 | 9.05 | 8.28 | 6.10 |
| Pyrazine | 9.28 | 5.71 | 7.01 | 8.10 | 8.62 | 8.94 | 7.96 | 5.84 |

Table S2: HOMO-LUMO gap [eV] for the molecules in the test set.

| molecule | BNL/3-21G | BNL/cc-pVDZ | BNL/cc-pVTZ | B3LYP/cc-pVTZ | PBE/cc-pVTZ | LC-DFTB | DFTB |
|---|---|---|---|---|---|---|---|
| Fluorene | 9.43 | 9.18 | 9.06 | 4.89 | 3.61 | 8.59 | 3.74 |
| PTCDA | 5.74 | 5.64 | 5.59 | 2.22 | 1.29 | 5.08 | 1.20 |
| $C_{60}$ | 6.41 | 6.20 | 6.15 | 2.61 | 1.60 | 5.80 | 1.80 |
| $H_2P$ | 5.85 | 5.92 | 5.91 | 2.83 | 1.88 | 5.24 | 1.68 |
| $H_2TPP$ | 5.31 | 5.33 | 5.32 | 2.44 | 1.57 | 4.74 | 1.44 |
| $H_2Pc$ | 5.07 | 4.89 | 4.80 | 2.11 | 1.40 | 4.38 | 1.31 |
| Benzothiazole | 9.83 | 9.65 | 9.55 | 5.26 | 3.86 | 7.91 | 3.68 |
| Benzothiadiazole | 8.24 | 8.13 | 8.04 | 3.77 | 2.51 | 6.64 | 2.49 |
| Thiadiazole | 10.64 | 10.30 | 10.10 | 5.43 | 3.89 | 7.72 | 3.25 |
| Thiophene | 11.01 | 10.77 | 10.62 | 5.95 | 4.49 | 8.45 | 4.02 |
| 2-Thiophene | 8.55 | 8.40 | 8.29 | 4.08 | 2.84 | 6.92 | 2.66 |
| 3-Thiophene | 7.49 | 7.37 | 7.28 | 3.30 | 2.19 | 6.15 | 2.10 |
| 5-Thiophene | 6.58 | 6.49 | 6.42 | 2.63 | 1.65 | 5.48 | 1.63 |
| 1-Acene | 11.69 | 11.36 | 11.20 | 6.63 | 5.14 | 10.80 | 5.28 |
| 2-Acene | 9.19 | 8.99 | 8.90 | 4.71 | 3.40 | 8.31 | 3.49 |
| 3-Acene | 7.58 | 7.44 | 7.37 | 3.48 | 2.31 | 6.80 | 2.44 |
| 4-Acene | 6.50 | 6.38 | 6.33 | 2.66 | 1.60 | 5.81 | 1.78 |
| 5-Acene | 5.73 | 5.62 | 5.58 | 2.09 | 1.12 | 5.14 | 1.33 |
| 6-Acene | 5.16 | 5.06 | 5.02 | 1.68 | 0.76 | 4.65 | 1.02 |
| Perylene | 6.75 | 6.62 | 6.55 | 2.89 | 1.84 | 6.05 | 2.02 |
| Coronene | 7.83 | 7.67 | 7.62 | 3.98 | 2.88 | 7.11 | 2.88 |
| NTCDA | 7.23 | 7.11 | 7.05 | 3.20 | 1.59 | 6.06 | 1.47 |
| Methane | 19.42 | 16.98 | 15.84 | 11.85 | 10.16 | 28.14 | 18.70 |
| Pyridine | 10.47 | 10.58 | 10.49 | 6.06 | 4.00 | 9.58 | 4.48 |
| Cyclopropene | 11.93 | 11.59 | 11.33 | 6.61 | 4.84 | 10.94 | 5.37 |
| Ketene | 10.50 | 10.63 | 10.62 | 5.73 | 3.84 | 10.39 | 1.20 |
| Dimethylether | 13.36 | 12.42 | 11.79 | 7.91 | 6.02 | 20.45 | 12.70 |
| Dimethylsulfide | 12.49 | 11.64 | 10.79 | 6.72 | 5.07 | 8.22 | 4.44 |
| Formaldehyde | 11.01 | 10.92 | 10.79 | 6.14 | 3.79 | 10.20 | 4.69 |
| Pyrene | 7.69 | 7.58 | 7.53 | 3.76 | 2.62 | 6.85 | 2.60 |
| 1,3-Butadiene | 10.44 | 10.23 | 10.10 | 5.50 | 3.99 | 9.39 | 4.15 |
| Propene | 12.45 | 12.06 | 11.80 | 7.02 | 5.33 | 11.62 | 5.83 |
| Pyridazine | 9.03 | 9.33 | 9.31 | 4.88 | 2.76 | 8.49 | 3.47 |
| Pyrimidine | 10.00 | 10.13 | 10.07 | 5.55 | 3.46 | 9.25 | 4.16 |
| Pyrazine | 9.66 | 9.81 | 9.73 | 5.27 | 3.21 | 8.49 | 3.70 |
